# Supplementary material for: Seeing Is Not Reaching: Instruction Shortcuts Override Visual Grounding in Vision-Language-Action Models
Source: arXiv:2611.32206 source file (2026-11-24)
Supplement: Supplementary file 1 [file A1_tabular.tex]

\begin{tabular}{l@{\hspace{6pt}}r rrrr@{\hspace{10pt}}rrrr}
\toprule
 & \multicolumn{5}{c}{LIBERO-PRO Position} & \multicolumn{4}{c}{Task-paired} \\
\cmidrule(lr){2-6}\cmidrule(lr){7-10}
Model & \mlh{$N$} & \mlh{requested\\object} & \mlh{training\\place} & \mlh{other training\\place (on the\\requested object)} & \mlh{elsewhere} & \mlh{place of\\the scene's\\task} & \mlh{requested\\object's\\training place} & \mlh{requested\\object} & \mlh{elsewhere} \\
\midrule
OpenVLA-OFT & 100 & 0 & 100 & 0 (0) & 0 & 100 & 0 & 0 & 0 \\
SmolVLA & 200 & 0 & 200 & 0 (0) & 0 & 167 & 30 & 0 & 3 \\
TurboVLA & 100 & 0 & 100 & 0 (0) & 0 & 100 & 0 & 0 & 0 \\
\piO-FAST & 200 & 0 & 199 & 0 (0) & 1 & 3 & 191 & 0 & 6 \\
\piO & 200 & 0 & 197 & 0 (0) & 3 & 0 & 197 & 0 & 3 \\
\piH & 200 & 28 & 121 & 14 (14) & 37 & 36 & 157 & 2 & 5 \\
\bottomrule
\end{tabular}
