# Supplementary material for: Seeing Is Not Reaching: Instruction Shortcuts Override Visual Grounding in Vision-Language-Action Models
Source: arXiv:2611.32206 source file (2026-11-24)
Supplement: Supplementary file 2 [file A1b_tabular.tex]

\begin{tabular}{lrrrr}
\toprule
Model & \mlw{$N$} & \mlw{object} & \mlw{req.\ train.} & \mlw{scene} \\
\midrule
OpenVLA-OFT & 50 & 0.76 & 0.64 & 0.71 \\
\piO & 50 & 0.22 & 0.57 & 0.48 \\
\piH & 50 & 4.50 & 2.30 & 1.00 \\
\bottomrule
\end{tabular}
