# Supplementary material for: Seeing Is Not Reaching: Instruction Shortcuts Override Visual Grounding in Vision-Language-Action Models
Source: arXiv:2611.32206 source file (2026-11-24)
Supplement: Supplementary file 3 [file A1n_tabular.tex]

\begin{tabular}{lrr}
\toprule
Model & \mlw{own} & \mlw{other} \\
\midrule
OpenVLA-OFT & 1.50 & 1.43 \\
SmolVLA & 1.30 & 1.29 \\
\piO-FAST & 1.23 & 0.63 \\
\piO & 0.79 & 0.85 \\
\piH & 6.38 & 1.30 \\
\bottomrule
\end{tabular}
