# Supplementary material for: Seeing Is Not Reaching: Instruction Shortcuts Override Visual Grounding in Vision-Language-Action Models
Source: arXiv:2611.32206 source file (2026-11-24)
Supplement: Supplementary file 4 [file float.tex]

\providecommand{\mlw}[1]{\makebox[2.6em][c]{\scriptsize\itshape #1}}
\begin{table*}[tp]
\centering
\footnotesize
\setlength\heavyrulewidth{0.25ex}
\captionsetup{position=top,skip=4pt}
\caption{\textbf{Under Position, five of the six VLAs first close at the requested object's training place in nearly every episode.}
First closes on the five LIBERO-Object tasks of \cref{supp:A3}, counts of $N$ episodes. The conservative criterion counts the \emph{requested object} column; the looser criterion adds the closes on the requested object where it stands on the other training place, in brackets under that place.}
\label{supp:A1}
\input{sec/suppl/A1/A1_tabular.tex}
\end{table*}
