# Supplementary material for: Seeing Is Not Reaching: Instruction Shortcuts Override Visual Grounding in Vision-Language-Action Models
Source: arXiv:2611.32206 source file (2026-11-24)
Supplement: Supplementary file 5 [file float.tex]

\begin{table*}[tp]
\centering
\footnotesize
\setlength\heavyrulewidth{0.25ex}
\captionsetup{position=top,skip=4pt}
\caption{\textbf{\boldmath Only \piH's name attention averages well above the image average, under the object's own name and on the requested object.}
(a) The attention of the requested object's name tokens on its main-camera patches, relative to the image average, under its own name (\emph{own}) and, on the same patches, when another object of the scene is named (\emph{other}); geometric mean over nine objects of each object's median over its moved scenes. SmolVLA's 64 visual tokens are read as an $8\times 8$ grid; name attention was not measured for TurboVLA.
(b) Name attention as in (a) on the first frame of the five Task-paired scenes, start states 0--9, with patches weighted by the object's pixels (so not on the scale of (a)). Columns: on the requested object (\emph{object}), on the object at its training place (\emph{req.\ train.}) and at the scene task's place (\emph{scene}); $N$: frames.}
\label{supp:A1n}
\begin{minipage}[t]{0.40\textwidth}\vspace{0pt}\centering
{\small (a)}\par\smallskip
\input{sec/suppl/A1/A1n_tabular.tex}
\end{minipage}\hspace{0.04\textwidth}%
\begin{minipage}[t]{0.40\textwidth}\vspace{0pt}\centering
{\small (b)}\par\smallskip
\setlength{\tabcolsep}{2.5pt}
\input{sec/suppl/A1/A1b_tabular.tex}
\end{minipage}
\end{table*}
