# Supplementary material for: Seeing Is Not Reaching: Instruction Shortcuts Override Visual Grounding in Vision-Language-Action Models
Source: arXiv:2611.32206 source file (2026-11-24)
Supplement: Supplementary file 6 [file float.tex]

\begin{figure*}[tp]
\centering
\includegraphics[width=\linewidth]{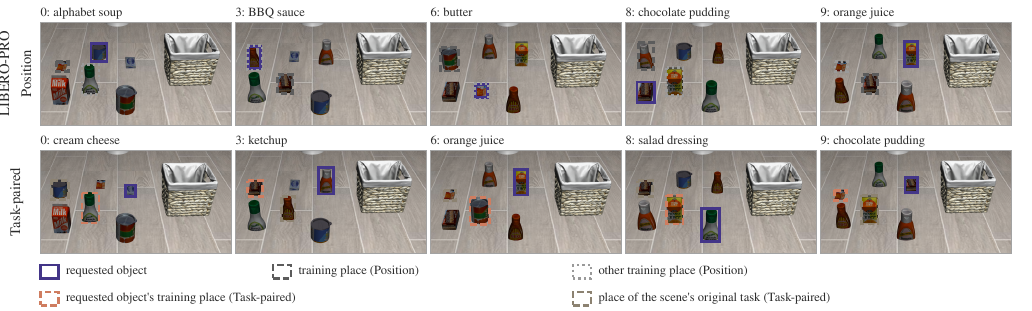}
\caption{\textbf{The places a first close is assigned to.}
The five LIBERO-Object tasks at start state 0, main camera, cropped to the objects; top: Position, bottom: Task-paired.
Each place is marked by the box of the object that stands there, as in the main paper's Fig.~1; in Position tasks 3 and 6 the requested object stands on the other training place, and its two boxes are drawn one inside the other.
}
\label{supp:A3}
\end{figure*}
