# Supplementary material for: Seeing Is Not Reaching: Instruction Shortcuts Override Visual Grounding in Vision-Language-Action Models
Source: arXiv:2611.32206 source file (2026-11-24)
Supplement: Supplementary file 7 [file A4_caption.tex]

\caption{\textbf{\boldmath For each of the eight other objects, \piH's name attention leaves the training place and lands on the new places.}
As in the main paper's Fig.~2(a), per main-camera patch: the change of the name's share of attention when the object moves from its training place to new places; the key is under the maps.
}
