# Supplementary material for: Seeing Is Not Reaching: Instruction Shortcuts Override Visual Grounding in Vision-Language-Action Models
Source: arXiv:2611.32206 source file (2026-11-24)
Supplement: Supplementary file 9 [file A5_caption.tex]

\caption{\textbf{\boldmath For every one of the nine objects, the \piH\ base model's name attention is above that of the \piO\ and \piO-FAST base models.}
As in the main paper's Fig.~2(b), per object: the name's attention on the moved object relative to the image average, median over its moved scenes; hollow markers: the object at its training place.
Stages: the vision-language model (PaliGemma 3B; Prismatic for OpenVLA), the robot-pretrained base (openpi's base checkpoints; OpenVLA 7B) and the LIBERO policy.
The last panel is the geometric mean over the nine objects; the vertical axis is logarithmic.
}
