# Supplementary material for: Seeing Is Not Reaching: Instruction Shortcuts Override Visual Grounding in Vision-Language-Action Models
Source: arXiv:2611.32206 source file (2026-11-24)
Supplement: Supplementary file 11 [file B0chk_caption.tex]

\caption{\textbf{Each cut removes exactly its connections: every check is 0 and every control above 0, in every episode.} Rows: each cut of the lower block of \cref{supp:B2}, and the cells of \cref{supp:G1} pooled. Columns: largest difference from the released policy; change from an instruction change with the cut (largest, must be 0) and without (smallest, above 0) (\cref{supp:protocol-text}); below, task 9's one-token length change under the direct cut, in normalized action units (\emph{$>$10\%}: above a tenth of the chunk's largest value).}
