# Supplementary material for: Seeing Is Not Reaching: Instruction Shortcuts Override Visual Grounding in Vision-Language-Action Models
Source: arXiv:2611.32206 source file (2026-11-24)
Supplement: Supplementary file 12 [file B0chk_tabular.tex]

\begin{tabular}{lllrcccc}
\toprule
 & & & & \multicolumn{2}{c}{\shortstack{mask off vs.\\ released}} & \multicolumn{2}{c}{\shortstack{instruction\\ change}} \\
\cmidrule(lr){5-6}\cmidrule(lr){7-8}
Model & Scenes & Cut & Ep. & \ml{chunk} & \ml{actions} & \ml{cut} & \ml{no cut} \\
\midrule
\piH & Position & no cut & 250 & 0 & 0 & -- & -- \\
 &  & grounding cut & 250 & 0 & 0 & 0 & 19.6 \\
 &  & direct cut & 250 & 0 & 0 & 0 & 1.54 \\
\addlinespace
 & original scenes & no cut & 250 & 0 & 0 & -- & -- \\
 &  & grounding cut & 250 & 0 & 0 & 0 & 15.8 \\
 &  & direct cut & 250 & 0 & 0 & 0 & 1.45 \\
\addlinespace
\piO & Position & no cut & 250 & 0 & 0 & -- & -- \\
 &  & grounding cut & 250 & 0 & 0 & 0 & 9.41 \\
 &  & direct cut & 250 & 0 & 0 & 0 & 1.05 \\
\midrule
\piH & Position & the cells of \cref{supp:G1} & 600 & 0 & 0 & 0 & 0.0571 \\
\bottomrule
\end{tabular}
