# Supplementary material for: Seeing Is Not Reaching: Instruction Shortcuts Override Visual Grounding in Vision-Language-Action Models
Source: arXiv:2611.32206 source file (2026-11-24)
Supplement: Supplementary file 13 [file float.tex]

\begin{table}[tbp]
\centering
\setlength\heavyrulewidth{0.25ex}
\scriptsize
\setlength{\tabcolsep}{2.8pt}
\captionsetup{position=top,skip=4pt}
\input{sec/suppl/B0chk/B0chk_caption.tex}
\label{supp:B0chk}
\input{sec/suppl/B0chk/B0chk_tabular.tex}

\vspace{6pt}
\input{sec/suppl/G1/G1len_tabular.tex}
\end{table}
