# Supplementary material for: Seeing Is Not Reaching: Instruction Shortcuts Override Visual Grounding in Vision-Language-Action Models
Source: arXiv:2611.32206 source file (2026-11-24)
Supplement: Supplementary file 14 [file float.tex]

\begin{figure*}[tp]
\centering
\begin{minipage}[b]{0.47\textwidth}\centering
\includegraphics[width=\linewidth]{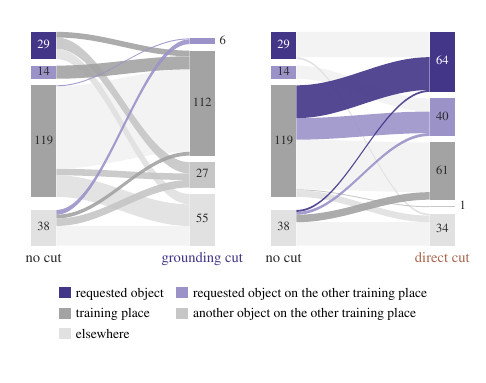}\\[2pt]
{\small (a)}
\end{minipage}\hfill
\begin{minipage}[b]{0.47\textwidth}\centering
\includegraphics[width=\linewidth]{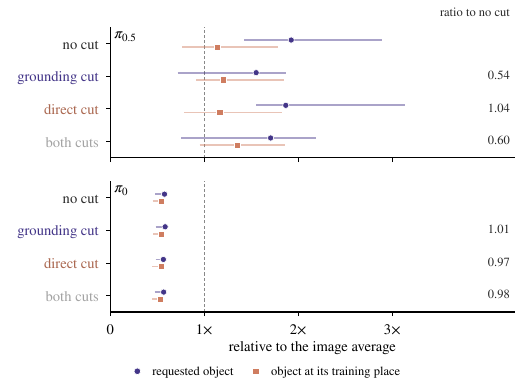}\\[2pt]
{\small (b)}
\end{minipage}
\caption{\textbf{\boldmath The two cuts move \piH's first closes in opposite directions; the grounding cut lowers its attention to the requested object and the direct cut does not.}
(a)~First closes with no cut and under each cut, the same episode paired across cuts; a ribbon that changes place takes the color of the place it arrives at.
(b)~Action-token attention to main-camera patches at the first query, relative to the image average, top \piH, bottom \piO; marker: median, bar: interquartile range; right: the median of each episode's ratio to no cut.
Under Position, 200 episodes per cut.}
\label{supp:B1}\label{supp:B6}
\end{figure*}
