# Supplementary material for: Seeing Is Not Reaching: Instruction Shortcuts Override Visual Grounding in Vision-Language-Action Models
Source: arXiv:2611.32206 source file (2026-11-24)
Supplement: Supplementary file 15 [file B2_tabular.tex]

\setlength{\tabcolsep}{3.0pt}
\begin{tabular}{llrrrrrcrr}
\toprule
 & & \multicolumn{5}{c}{LIBERO-PRO Position} & & \multicolumn{2}{c}{Original scenes} \\
\cmidrule(lr){3-7}\cmidrule(lr){9-10}
Model & Cut & {\scriptsize\itshape \mlh{requested\\object}} & {\scriptsize\itshape \mlh{training\\place}} & {\scriptsize\itshape \mlh{other training\\place (on the\\requested object)}} & {\scriptsize\itshape \mlh{elsewhere}} & {\scriptsize\itshape \mlh{succ.}} & & {\scriptsize\itshape \mlh{requested\\object}} & {\scriptsize\itshape \mlh{succ.}} \\
\midrule
\piH & no cut & 29 & 119 & 14 (14) & 38 & 15 & & 200 & 196 \\
 & grounding cut & 0 & 112 & 33 (6) & 55 & 5 & & -- & -- \\
 & direct cut & 64 & 61 & 41 (40) & 34 & 81 & & 199 & 196 \\
 & both cuts & 4 & 86 & 74 (7) & 36 & 8 & & -- & -- \\
 & grounding cut ($N_r$) & 0 & 119 & 39 (3) & 42 & 3 & & -- & -- \\
 & direct cut ($N_r$) & 30 & 120 & 17 (17) & 33 & 23 & & -- & -- \\
 & both cuts ($N_r$) & 0 & 115 & 40 (3) & 45 & 3 & & -- & -- \\
\midrule
\piO & no cut & 0 & 197 & 0 (0) & 3 & 0 & & 200 & 188 \\
 & grounding cut & 0 & 126 & 72 (31) & 2 & 22 & & -- & -- \\
 & direct cut & 0 & 198 & 0 (0) & 2 & 0 & & 199 & 181 \\
 & both cuts & 2 & 128 & 69 (25) & 1 & 19 & & -- & -- \\
 & grounding cut ($N_r$) & 0 & 162 & 38 (11) & 0 & 6 & & -- & -- \\
 & direct cut ($N_r$) & 0 & 195 & 0 (0) & 5 & 0 & & -- & -- \\
 & both cuts ($N_r$) & 0 & 159 & 41 (11) & 0 & 6 & & -- & -- \\
\midrule
\multicolumn{10}{l}{\itshape Repeat, 250 episodes per cut} \\
\piH & no cut & 35 & 154 & 25 (25) & 36 & 37 & & 250 & 246 \\
 & grounding cut & 0 & 140 & 54 (9) & 56 & 10 & & 213 & 210 \\
 & direct cut & 71 & 91 & 53 (50) & 35 & 95 & & 249 & 247 \\
\midrule
\piO & no cut & 0 & 236 & 0 (0) & 14 & 0 & & -- & -- \\
 & grounding cut & 2 & 135 & 111 (39) & 2 & 31 & & -- & -- \\
 & direct cut & 0 & 237 & 0 (0) & 13 & 0 & & -- & -- \\
\bottomrule
\end{tabular}
