# Supplementary material for: Seeing Is Not Reaching: Instruction Shortcuts Override Visual Grounding in Vision-Language-Action Models
Source: arXiv:2611.32206 source file (2026-11-24)
Supplement: Supplementary file 16 [file float.tex]

\begin{table*}[tp]
\centering
\setlength\heavyrulewidth{0.25ex}
\footnotesize
\captionsetup{position=top,skip=4pt}
\caption{\textbf{Every pathway cut under LIBERO-PRO Position: in \piH\ the grounding cut takes away the reaches and the direct cut adds them, and the repeat on 250 episodes per cut gives the same.}
Upper block: each cut, 200 episodes per cell (no cut: \cref{supp:protocol-text}); lower block: the repeat, 250 episodes per cell; Position columns as in \cref{supp:A1}; $N_r$: restricted to the requested object's name. \emph{succ.}: successes; --: not run.
}
\label{supp:B2}
\input{sec/suppl/B2/B2_tabular.tex}
\end{table*}
