# Supplementary material for: Seeing Is Not Reaching: Instruction Shortcuts Override Visual Grounding in Vision-Language-Action Models
Source: arXiv:2611.32206 source file (2026-11-24)
Supplement: Supplementary file 17 [file float.tex]

\begin{figure*}[tp]
\centering
\includegraphics[width=\linewidth]{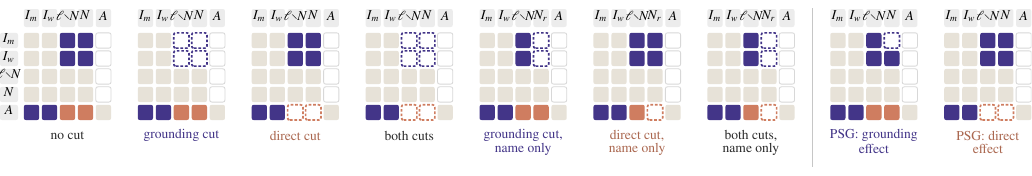}
\caption{\textbf{The attention masks of the pathway cuts and of PSG.}
Left: the seven conditions of the pathway cuts. Right: the two masks PSG evaluates at every Euler step, one for the grounding effect and one for the direct effect.
Rows attend to columns; dashed cells are masked in every layer and head. $I_m$, $I_w$: main- and wrist-camera image tokens; $N$: PSG's name tokens; $N_r$: the requested object's name; $\ell{\setminus}N$: the other instruction tokens; $A$: action tokens. Drawn for \piH; in \piO\ the state token is masked with the action tokens.
}
\label{supp:B5}
\end{figure*}
