# Supplementary material for: Seeing Is Not Reaching: Instruction Shortcuts Override Visual Grounding in Vision-Language-Action Models
Source: arXiv:2611.32206 source file (2026-11-24)
Supplement: Supplementary file 18 [file float.tex]

\begin{figure*}[tp]
\centering
\includegraphics[width=\linewidth]{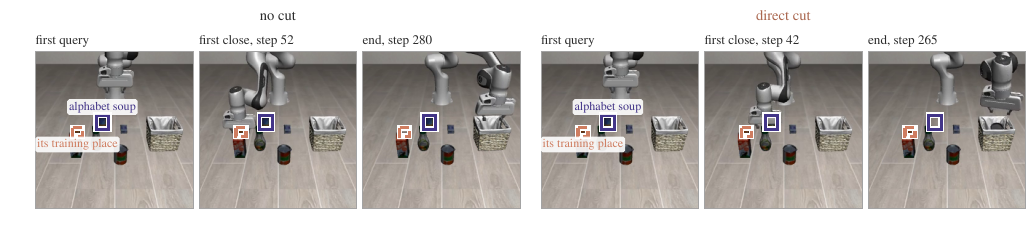}
\caption{\textbf{\boldmath Under the direct cut, \piH's hand closes on the moved alphabet soup instead of at its training place.}
One episode of Position task 0 (the alphabet soup, the requested object), main camera, with no cut and under the direct cut (same start state and noise seed); boxes: the requested object and its training place.
}
\label{supp:B7}
\end{figure*}
