# Supplementary material for: Seeing Is Not Reaching: Instruction Shortcuts Override Visual Grounding in Vision-Language-Action Models
Source: arXiv:2611.32206 source file (2026-11-24)
Supplement: Supplementary file 19 [file C3_caption.tex]

\caption{\textbf{PSG adds Reach where the object's own name draws the attention; for the BBQ sauce, whose name does not, it adds none.} Five LIBERO-Object objects under Position: the own-name ratio (the name's attention under its own name over the strongest under another object's name; median and range over ten frames) against what PSG adds to \piH's Reach on the object's task, 50 episodes per task. Reach by the looser criterion, since in tasks 3 and 6 the requested object stands on the other training place.}
