# Supplementary material for: Seeing Is Not Reaching: Instruction Shortcuts Override Visual Grounding in Vision-Language-Action Models
Source: arXiv:2611.32206 source file (2026-11-24)
Supplement: Supplementary file 20 [file float.tex]

\begin{figure}[tbp]
\centering
\includegraphics[width=\linewidth]{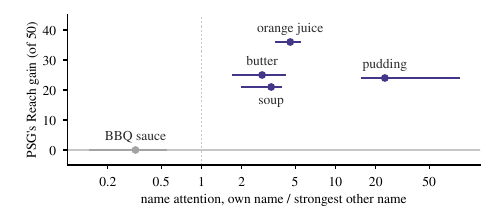}
\input{sec/suppl/C3/C3_caption.tex}
\label{supp:C3}
\end{figure}
