# Supplementary material for: Seeing Is Not Reaching: Instruction Shortcuts Override Visual Grounding in Vision-Language-Action Models
Source: arXiv:2611.32206 source file (2026-11-24)
Supplement: Supplementary file 21 [file C4p2_caption.tex]

\caption{\textbf{Over the ten LIBERO-PRO Position Object tasks, each of PSG's two effects alone raises Reach, the two together give the most successes, and the gain holds at every tested $a$.} Counts of episodes, 20 per task and row, on start states the selection did not use; \emph{dev.}: the three development tasks; the two weights act on the six motion dimensions of PSG's sampler (Algorithm~\ref{alg:psg}).}
