# Supplementary material for: Seeing Is Not Reaching: Instruction Shortcuts Override Visual Grounding in Vision-Language-Action Models
Source: arXiv:2611.32206 source file (2026-11-24)
Supplement: Supplementary file 22 [file C4p2_tabular.tex]

\begin{tabular}{@{}lrrrrrrrr@{}}
\toprule
 & & & \multicolumn{2}{c}{all (200)} & \multicolumn{2}{c}{dev. (60)} & \multicolumn{2}{c}{other (140)} \\
\cmidrule(lr){4-5}\cmidrule(lr){6-7}\cmidrule(lr){8-9}
Setting & $a$ & $b$ & \ml{Reach} & \ml{Succ.} & \ml{Reach} & \ml{Succ.} & \ml{Reach} & \ml{Succ.} \\
\midrule
released \piH & -- & -- & 42 & 33 & 18 & 13 & 24 & 20 \\
grounding removed & $-1$ & 0 & 23 & 22 & 2 & 2 & 21 & 20 \\
direct removed & 0 & 1 & 75 & 58 & 43 & 33 & 32 & 25 \\
grounding amplified & 5 & 0 & 89 & 52 & 34 & 27 & 55 & 25 \\
weight $a = 1$ & 1 & 1 & 98 & 78 & 48 & 47 & 50 & 31 \\
weight $a = 2$ & 2 & 1 & 103 & 83 & 48 & 46 & 55 & 37 \\
\rowcolor[HTML]{EDEDED}PSG & 5 & 1 & 105 & 84 & 47 & 44 & 58 & 40 \\
weight $a = 8$ & 8 & 1 & 107 & 81 & 47 & 37 & 60 & 44 \\
\bottomrule
\end{tabular}
