# Supplementary material for: Seeing Is Not Reaching: Instruction Shortcuts Override Visual Grounding in Vision-Language-Action Models
Source: arXiv:2611.32206 source file (2026-11-24)
Supplement: Supplementary file 23 [file C4p2fig_caption.tex]

\caption{\textbf{With PSG's grounding effect removed, the hand first closes on the object at the requested object's training place in 19 or 20 of 20 episodes in six of the ten tasks.} One panel per task, one bar per row for the first four settings of \cref{supp:C4p2} and PSG, 20 episodes per bar; bold: the three development tasks; outlined: the row with the grounding effect removed. Hatched: the object at the slot beside the training place.}
