# Supplementary material for: Seeing Is Not Reaching: Instruction Shortcuts Override Visual Grounding in Vision-Language-Action Models
Source: arXiv:2611.32206 source file (2026-11-24)
Supplement: Supplementary file 26 [file C5_tabular.tex]

\begin{tabular}{lrrrrrr}
\toprule
 & \multicolumn{2}{c}{all (500)} & \multicolumn{2}{c}{conservative (250)} & \multicolumn{2}{c}{held out (280)}\\
\cmidrule(lr){2-3}\cmidrule(lr){4-5}\cmidrule(lr){6-7}
Method & \ml{Reach} & \ml{Succ.} & \ml{Reach} & \ml{Succ.} & \ml{Reach} & \ml{Succ.}\\
\midrule
\piH & 22.0 & 16.6 & 14.0 & 8.8 & 18.2 & 13.9\\
\ + CAG & 26.6 & 16.4 & 20.8 & 6.0 & 27.9 & 17.1\\
\rowcolor[HTML]{EDEDED}\ + PSG & 52.6 & 40.8 & 46.4 & 25.2 & 42.5 & 28.2\\
\bottomrule
\end{tabular}
