# Supplementary material for: Seeing Is Not Reaching: Instruction Shortcuts Override Visual Grounding in Vision-Language-Action Models
Source: arXiv:2611.32206 source file (2026-11-24)
Supplement: Supplementary file 27 [file float.tex]

\begin{table}[tp]
\centering
\footnotesize
\setlength\heavyrulewidth{0.25ex}
\setlength{\tabcolsep}{3pt}
\captionsetup{position=top,skip=4pt}
\caption{\textbf{\boldmath On LIBERO-PRO Position Object, PSG raises \piH's Reach and success on all episodes, on the five tasks the conservative criterion counts, and on the episodes held out from the selection of its weights.}
Columns: the episodes of the main paper's Tab.~1; those of the five tasks whose requested object does not stand on the other training place; those that share no task and no start state with the selection; episodes in brackets.}
\label{supp:C5}
\input{sec/suppl/C5/C5_tabular.tex}
\end{table}
