# Supplementary material for: Seeing Is Not Reaching: Instruction Shortcuts Override Visual Grounding in Vision-Language-Action Models
Source: arXiv:2611.32206 source file (2026-11-24)
Supplement: Supplementary file 28 [file C6_caption.tex]

\caption{\textbf{\boldmath On Position Object, PSG's gain repeats with a second noise seed. In the control on \piO, whose name attention stays near the image average, the same sampler leaves Reach at 1.2\%.}
500 episodes per row; \emph{conservative}: Reach on the conservative criterion's five tasks; \emph{gained}, \emph{lost}: episodes in which PSG has a reach and the row above has none, and the reverse, paired by task and start state.}
