# Supplementary material for: Seeing Is Not Reaching: Instruction Shortcuts Override Visual Grounding in Vision-Language-Action Models
Source: arXiv:2611.32206 source file (2026-11-24)
Supplement: Supplementary file 29 [file C6_tabular.tex]

\begin{tabular}{lrrrrr}
\toprule
Method & \ml{Reach} & {\scriptsize\itshape conservative} & \ml{Succ.} & \ml{gained} & \ml{lost}\\
\midrule
\piH, seed 7 & 22.0 & 14.0 & 16.6 &  & \\
\rowcolor[HTML]{EDEDED}\ + PSG & 52.6 & 46.4 & 40.8 & 153 & 0\\
\midrule
\piH, seed 17 & 22.6 & 15.6 & 17.2 &  & \\
\rowcolor[HTML]{EDEDED}\ + PSG & 51.4 & 43.6 & 39.2 & 147 & 3\\
\midrule
\piO, seed 7 & 0.0 & 0.0 & 0.2 &  & \\
\rowcolor[HTML]{EDEDED}\ + PSG & 1.2 & 2.0 & 0.0 & 6 & 0\\
\bottomrule
\end{tabular}
