# Supplementary material for: Seeing Is Not Reaching: Instruction Shortcuts Override Visual Grounding in Vision-Language-Action Models
Source: arXiv:2611.32206 source file (2026-11-24)
Supplement: Supplementary file 30 [file float.tex]

\begin{table}[tp]
\centering
\footnotesize
\setlength\heavyrulewidth{0.25ex}
\setlength{\tabcolsep}{4pt}
\captionsetup{position=top,skip=4pt}
\input{sec/suppl/C6/C6_caption.tex}
\label{supp:C6}
\input{sec/suppl/C6/C6_tabular.tex}
\end{table}
