# Supplementary material for: Seeing Is Not Reaching: Instruction Shortcuts Override Visual Grounding in Vision-Language-Action Models
Source: arXiv:2611.32206 source file (2026-11-24)
Supplement: Supplementary file 31 [file D1f2_tabular.tex]

\footnotesize
\setlength{\tabcolsep}{2.4pt}
\begin{tabular}{lr@{\hspace{1.5pt}}r@{\hspace{6pt}}>{\color{black!55}}r@{\hspace{1.5pt}}>{\color{black!55}}r@{\hspace{6pt}}r@{\hspace{1.5pt}}r@{\hspace{6pt}}>{\columncolor[HTML]{EDEDED}[3pt][0.75pt]}r@{\hspace{1.5pt}}>{\columncolor[HTML]{EDEDED}[0.75pt][3pt]}r}
\toprule
Task & \multicolumn{2}{c}{\piH} & \multicolumn{2}{c}{+\,CAG-VA$^\dagger$} & \multicolumn{2}{c}{+\,CAG} & \multicolumn{2}{c}{+\,PSG}\\
\cmidrule(lr){2-3}\cmidrule(lr){4-5}\cmidrule(lr){6-7}\cmidrule(lr){8-9}
 & {\scriptsize\itshape R} & {\scriptsize\itshape S} & {\scriptsize\itshape R} & {\scriptsize\itshape S} & {\scriptsize\itshape R} & {\scriptsize\itshape S} & {\scriptsize\itshape R} & {\scriptsize\itshape S}\\
\midrule
\multicolumn{9}{l}{\textit{LIBERO-CF Object}}\\
\parbox[t]{7.2cm}{\raggedright 01 pick up the cream cheese and place it in the basket} & 8 & 10 & 26 & 24 & 20 & 18 & 46 & 28\\
\parbox[t]{7.2cm}{\raggedright 02 pick up the butter and place it in the basket} & 0 & 0 & 0 & 0 & 0 & 0 & 0 & 0\\
\parbox[t]{7.2cm}{\raggedright 03 pick up the tomato sauce and place it in the basket} & 0 & 0 & 0 & 0 & 0 & 0 & 0 & 0\\
\parbox[t]{7.2cm}{\raggedright 04 pick up the salad dressing and place it in the basket} & 24 & 20 & 46 & 30 & 34 & 28 & 52 & 18\\
\parbox[t]{7.2cm}{\raggedright 05 pick up the milk and place it in the basket} & 0 & 0 & 0 & 0 & 0 & 0 & 0 & 0\\
\parbox[t]{7.2cm}{\raggedright 06 pick up the bbq sauce and place it in the basket} & 0 & 0 & 0 & 0 & 0 & 0 & 0 & 0\\
\parbox[t]{7.2cm}{\raggedright 07 pick up the ketchup and place it in the basket} & 14 & 2 & 28 & 4 & 22 & 4 & 28 & 6\\
\parbox[t]{7.2cm}{\raggedright 08 pick up the orange juice and place it in the basket} & 0 & 0 & 64 & 32 & 34 & 12 & 88 & 10\\
\parbox[t]{7.2cm}{\raggedright 09 pick up the alphabet soup and place it in the basket} & 28 & 24 & 62 & 48 & 26 & 22 & 70 & 62\\
\parbox[t]{7.2cm}{\raggedright 10 pick up the chocolate pudding and place it in the basket} & 0 & 0 & 0 & 0 & 0 & 0 & 0 & 4\\
\parbox[t]{7.2cm}{\raggedright \textbf{all tasks}} & 7.4 & 5.6 & 22.6 & 13.8 & 13.6 & 8.4 & 28.4 & 12.8\\
\bottomrule
\end{tabular}
