# Supplementary material for: Seeing Is Not Reaching: Instruction Shortcuts Override Visual Grounding in Vision-Language-Action Models
Source: arXiv:2611.32206 source file (2026-11-24)
Supplement: Supplementary file 32 [file D1f3_tabular.tex]

\footnotesize
\setlength{\tabcolsep}{2.4pt}
\begin{tabular}{lr@{\hspace{1.5pt}}r@{\hspace{6pt}}>{\color{black!55}}r@{\hspace{1.5pt}}>{\color{black!55}}r@{\hspace{6pt}}r@{\hspace{1.5pt}}r@{\hspace{6pt}}>{\columncolor[HTML]{EDEDED}[3pt][0.75pt]}r@{\hspace{1.5pt}}>{\columncolor[HTML]{EDEDED}[0.75pt][3pt]}r}
\toprule
Task & \multicolumn{2}{c}{\piH} & \multicolumn{2}{c}{+\,CAG-VA$^\dagger$} & \multicolumn{2}{c}{+\,CAG} & \multicolumn{2}{c}{+\,PSG}\\
\cmidrule(lr){2-3}\cmidrule(lr){4-5}\cmidrule(lr){6-7}\cmidrule(lr){8-9}
 & {\scriptsize\itshape R} & {\scriptsize\itshape S} & {\scriptsize\itshape R} & {\scriptsize\itshape S} & {\scriptsize\itshape R} & {\scriptsize\itshape S} & {\scriptsize\itshape R} & {\scriptsize\itshape S}\\
\midrule
\multicolumn{9}{l}{\textit{LIBERO-CF OOD}}\\
\parbox[t]{7.2cm}{\raggedright 01 pick up the coke can and place it on the plate} & 16 & 6 & 28 & 18 & 10 & 8 & 44 & 34\\
\parbox[t]{7.2cm}{\raggedright 02 pick up the coke can and place it on the plate} & 0 & 0 & 14 & 14 & 4 & 4 & 4 & 2\\
\parbox[t]{7.2cm}{\raggedright 03 pick up the coke can and place it on the plate} & 46 & 34 & 66 & 34 & 52 & 44 & 58 & 42\\
\parbox[t]{7.2cm}{\raggedright 04 pick up the cup and place it on the plate} & 2 & 0 & 8 & 6 & 0 & 2 & 0 & 0\\
\parbox[t]{7.2cm}{\raggedright 05 pick up the cup and place it on the plate} & 16 & 16 & 20 & 18 & 16 & 16 & 16 & 16\\
\parbox[t]{7.2cm}{\raggedright 06 pick up the cup and place it on the plate} & 6 & 2 & 12 & 6 & 4 & 2 & 4 & 4\\
\parbox[t]{7.2cm}{\raggedright 07 pick up the beer and place it on the plate} & 0 & 0 & 8 & 2 & 0 & 0 & 0 & 0\\
\parbox[t]{7.2cm}{\raggedright 08 pick up the beer and place it on the plate} & 4 & 0 & 22 & 0 & 24 & 2 & 14 & 4\\
\parbox[t]{7.2cm}{\raggedright 09 pick up the beer and place it on the plate} & 24 & 2 & 34 & 8 & 18 & 0 & 12 & 4\\
\parbox[t]{7.2cm}{\raggedright 10 pick up the apple and place it on the plate} & 0 & 0 & 2 & 2 & 0 & 0 & 2 & 0\\
\parbox[t]{7.2cm}{\raggedright 11 pick up the apple and place it on the plate} & 6 & 0 & 10 & 4 & 6 & 0 & 4 & 0\\
\parbox[t]{7.2cm}{\raggedright 12 pick up the apple and place it on the plate} & 0 & 0 & 0 & 0 & 0 & 0 & 8 & 2\\
\parbox[t]{7.2cm}{\raggedright 13 pick up the banana and place it on the plate} & 58 & 38 & 98 & 46 & 84 & 72 & 98 & 48\\
\parbox[t]{7.2cm}{\raggedright 14 pick up the banana and place it on the plate} & 2 & 0 & 22 & 2 & 12 & 6 & 44 & 6\\
\parbox[t]{7.2cm}{\raggedright 15 pick up the banana and place it on the plate} & 52 & 0 & 74 & 0 & 50 & 6 & 74 & 0\\
\parbox[t]{7.2cm}{\raggedright \textbf{all tasks}} & 15.5 & 6.5 & 27.9 & 10.7 & 18.7 & 10.8 & 25.5 & 10.8\\
\bottomrule
\end{tabular}
