# Supplementary material for: Seeing Is Not Reaching: Instruction Shortcuts Override Visual Grounding in Vision-Language-Action Models
Source: arXiv:2611.32206 source file (2026-11-24)
Supplement: Supplementary file 33 [file float.tex]

\begin{table*}[tp]
\centering
\setlength\heavyrulewidth{0.25ex}
\ContinuedFloat
\captionsetup{position=top,skip=4pt}
\caption[]{(continued)}
\input{sec/suppl/D1/D1f2_tabular.tex}
\par\medskip
\input{sec/suppl/D1/D1f3_tabular.tex}
\end{table*}
