# Supplementary material for: Seeing Is Not Reaching: Instruction Shortcuts Override Visual Grounding in Vision-Language-Action Models
Source: arXiv:2611.32206 source file (2026-11-24)
Supplement: Supplementary file 34 [file D2_caption.tex]

\caption{\textbf{The test sets of the main paper's tables.} One line per test set: its tasks, start states and noise seeds, the episodes of each row, the step limit, how Reach is decided, and the table that uses it. Target object moved: our scenes, each object at its training place and at new places named by grid cell (the Object line is the Object grid of \cref{supp:C2}).}
