# Supplementary material for: Seeing Is Not Reaching: Instruction Shortcuts Override Visual Grounding in Vision-Language-Action Models
Source: arXiv:2611.32206 source file (2026-11-24)
Supplement: Supplementary file 35 [file D2_tabular.tex]

\footnotesize
\setlength{\tabcolsep}{3pt}
\begin{tabular}{l>{\raggedright\arraybackslash}p{2.1cm}rllrl>{\raggedright\arraybackslash}p{3.3cm}l}
\toprule
Benchmark & Suite & \ml{tasks} & \ml{states} & \ml{seeds} & \ml{ep./row} & \ml{steps} & Reach rule & \ml{tab.}\\
\midrule
LIBERO & Spatial & 10 & 0--49 & 7 & 500 & 220 & -- & 1\\
LIBERO & Object & 10 & 0--49 & 7 & 500 & 280 & -- & 1\\
LIBERO & Goal & 10 & 0--49 & 7 & 500 & 300 & -- & 1\\
LIBERO & Long & 10 & 0--49 & 7 & 500 & 520 & -- & 1\\
LIBERO-PRO Position & Object & 10 & 0--49 & 7 & 500 & 280 & first close 10 & 1\\
LIBERO-PRO Position & Goal & 10 & 0--49 & 7 & 500 & 300 & first close 6; first contact 4 & 1\\
LIBERO-PRO Position & Spatial & 10 & 0--49 & 7 & 500 & 220 & first close 10 & 1\\
LIBERO-PRO Task & Object & 10 & 0--49 & 7 & 500 & 280 & first close 10 & 1\\
LIBERO-PRO Task & Goal & 10 & 0--49 & 7 & 500 & 300 & first close 6; first contact 4 & 1\\
LIBERO-PRO Task & Spatial & 10 & 0--49 & 7 & 500 & 220 & first close 10 & 1\\
LIBERO-Plus Layout & all four & 1525 & 0 & 7 & 1525 & 220/280/300/520 & first close 1316; first contact 209 & 1\\
LIBERO, target object moved & Object (the Object grid) & 70 & 6--15 & 7 & 689 & 280 & first close 70 & --\\
LIBERO, target object moved & Goal & 21 & 6--15 & 7 & 210 & 300 & first close 21 & 2\\
LIBERO-CF & Spatial & 15 & 0--49 & 7 & 750 & 220 & first close 15 & 3\\
LIBERO-CF & Object & 10 & 0--49 & 7 & 500 & 280 & first close 10 & 3\\
LIBERO-CF & OOD & 15 & 0--49 & 7 & 750 & 220 & first close 15 & 3\\
\bottomrule
\end{tabular}
