# Supplementary material for: Seeing Is Not Reaching: Instruction Shortcuts Override Visual Grounding in Vision-Language-Action Models
Source: arXiv:2611.32206 source file (2026-11-24)
Supplement: Supplementary file 36 [file float.tex]

\begin{table*}[tp]
\centering
\setlength\heavyrulewidth{0.25ex}
\captionsetup{position=top,skip=4pt}
\input{sec/suppl/D2/D2_caption.tex}
\label{supp:D2}
\input{sec/suppl/D2/D2_tabular.tex}
\end{table*}
