# Supplementary material for: Seeing Is Not Reaching: Instruction Shortcuts Override Visual Grounding in Vision-Language-Action Models
Source: arXiv:2611.32206 source file (2026-11-24)
Supplement: Supplementary file 37 [file D3_tabular.tex]

\footnotesize
\setlength{\tabcolsep}{2pt}
\begin{tabular}{llllll}
\toprule
Method & Built on & Checkpoint & Version & Inference settings & LIBERO Avg\\
\midrule
OpenVLA-OFT & \parbox[t]{1.9cm}{\raggedright its own release\strut} & \texttt{libero-spatial-object-goal-10} & {\ttfamily 638918f3d1} & \parbox[t]{3.4cm}{\raggedright L1 regression, parallel decoding; chunk 8, 8 executed per replan\strut} & reported\\
SmolVLA & \parbox[t]{1.9cm}{\raggedright its own release\strut} & \texttt{smolvla\_libero} & {\ttfamily a24f1f3804} & \parbox[t]{3.4cm}{\raggedright Euler, 10 steps, t from 1 to 0; chunk 50, 10 executed per replan\strut} & reported\\
TurboVLA & \parbox[t]{1.9cm}{\raggedright its own release\strut} & \texttt{TurboVLA} & {\ttfamily 9cdb576ed9} & \parbox[t]{3.4cm}{\raggedright one forward pass, ACT queries, tanh; chunk 12, 12 executed per replan\strut} & reported\\
\piO-FAST & \parbox[t]{1.9cm}{\raggedright its own release\strut} & \texttt{pi0\_fast\_libero} & {\ttfamily d59b9cc921} & \parbox[t]{3.4cm}{\raggedright autoregressive, temperature 0.0; chunk 10, 5 executed per replan\strut} & reported\\
\piO & \parbox[t]{1.9cm}{\raggedright its own release\strut} & \texttt{pi0\_libero} & {\ttfamily 20205f127b} & \parbox[t]{3.4cm}{\raggedright flow matching, 10 Euler steps; chunk 50, 5 executed per replan\strut} & reported\\
RSS$^\dagger$ & \parbox[t]{1.9cm}{\raggedright the authors' own fine-tune of \piH\strut} & \texttt{RSS\_pi05\_cfg\_libero\_caption} & {\ttfamily d992b3fe7b} & \parbox[t]{3.4cm}{\raggedright Euler; 10 steps; chunk 10, 5 executed per replan; guidance scale 1.5\strut} & reported\\
APT$^\dagger$ & \parbox[t]{1.9cm}{\raggedright Qwen3-VL-2B-Instruct (frozen) and a LIBERO fine-tune\strut} & \texttt{apt\_models} & {\ttfamily cd98ada16d} & \parbox[t]{3.4cm}{\raggedright DDIM; 20 steps; 3 actions per model call\strut} & reported\\
\piH & \parbox[t]{1.9cm}{\raggedright its own release\strut} & \texttt{pi05\_libero} & {\ttfamily 42d571bd87} & \parbox[t]{3.4cm}{\raggedright flow matching, 10 Euler steps; chunk 10, 5 executed per replan\strut} & measured\\
\piH\ + CAG & \parbox[t]{1.9cm}{\raggedright the released \piH\strut} & \texttt{pi05\_libero} & {\ttfamily 42d571bd87} & \parbox[t]{3.4cm}{\raggedright Euler; 10 steps; chunk 10, 5 executed per replan; guidance scale 1.5\strut} & measured\\
\piH\ + CAG-VA$^\dagger$ & \parbox[t]{1.9cm}{\raggedright the released \piH\ and CAG's vision-action model\strut} & \texttt{pi05\_libero} + \texttt{pi05-libero-VA} & {\ttfamily 42d571bd87} & \parbox[t]{3.4cm}{\raggedright Euler; 10 steps; chunk 10, 5 executed per replan; guidance scale 1.5\strut} & --\\
\rowcolor[HTML]{EDEDED}\piH\ + PSG (Ours) & \parbox[t]{1.9cm}{\raggedright the released \piH\strut} & \texttt{pi05\_libero} & {\ttfamily 42d571bd87} & \parbox[t]{3.4cm}{\raggedright flow matching, 10 Euler steps; chunk 10, 5 executed per replan; a = 5, b = 1\strut} & measured\\
\bottomrule
\end{tabular}
