# Supplementary material for: Seeing Is Not Reaching: Instruction Shortcuts Override Visual Grounding in Vision-Language-Action Models
Source: arXiv:2611.32206 source file (2026-11-24)
Supplement: Supplementary file 38 [file float.tex]

\begin{table*}[tp]
\centering
\setlength\heavyrulewidth{0.25ex}
\captionsetup{position=top,skip=4pt}
\caption{\textbf{Compared methods, and the checkpoints behind the main paper's Fig.~1.} Each row's base model, checkpoint and the inference settings it ran with in every test set (\cref{supp:D2}); \emph{LIBERO Avg}: whether the main paper's Tab.~1 gives the LIBERO average as measured here or as reported (for \piO-FAST and \piO\ in openpi's LIBERO README, for the others in the method's own paper). $\dagger$: requires training; --: not run on LIBERO (CAG-VA ran only on LIBERO-CF). Below: the checkpoints of the main paper's Fig.~1; OpenVLA-OFT and TurboVLA there are their LIBERO-Object checkpoints.}
\label{supp:D3}
\input{sec/suppl/D3/D3_tabular.tex}
\par\medskip
{\footnotesize\itshape The checkpoints behind the main paper's Fig.~1}\par\smallskip
{\footnotesize\setlength{\tabcolsep}{3pt}\input{sec/suppl/D3runs/D3ck_tabular.tex}}
\end{table*}
