# Supplementary material for: Seeing Is Not Reaching: Instruction Shortcuts Override Visual Grounding in Vision-Language-Action Models
Source: arXiv:2611.32206 source file (2026-11-24)
Supplement: Supplementary file 39 [file D3ck_tabular.tex]

\begin{tabular}{@{}l>{\raggedright\arraybackslash}p{4.3cm}l@{}}
\toprule
Model & Checkpoint & Version \\
\midrule
OpenVLA-OFT & \texttt{openvla-\allowbreak{}7b-\allowbreak{}oft-\allowbreak{}finetuned-\allowbreak{}libero-\allowbreak{}object} & 4c89574e \\
SmolVLA & \texttt{smolvla\_libero} & 31d453f7 \\
TurboVLA & \texttt{TurboVLA, object.pth} & f7b0f53a \\
\piO-FAST & \texttt{pi0\_fast\_libero} & d59b9cc9 \\
\piO & \texttt{pi0\_libero} & 20205f12 \\
\piH & \texttt{pi05\_libero} & 42d571bd \\
\bottomrule
\end{tabular}
