# Supplementary material for: Seeing Is Not Reaching: Instruction Shortcuts Override Visual Grounding in Vision-Language-Action Models
Source: arXiv:2611.32206 source file (2026-11-24)
Supplement: Supplementary file 40 [file D3settings_tabular.tex]

\begin{tabular}{@{}>{\raggedright\arraybackslash}p{3.6cm}>{\raggedright\arraybackslash}p{1.9cm}>{\raggedright\arraybackslash}p{3.4cm}>{\raggedright\arraybackslash}p{1.6cm}>{\raggedright\arraybackslash}p{2.1cm}>{\raggedright\arraybackslash}p{2.6cm}r@{}}
\toprule
Figure or table & Models & Scenes & Start states & Noise seeds & Episodes & Steps \\
\midrule
main Fig.~1; \cref{supp:A1} & 6 VLAs & Position, Task-paired; Object tasks 0, 3, 6, 8, 9 & 0--19 & 7, 17 (OpenVLA-OFT, TurboVLA: 7) & 200 per test (OpenVLA-OFT, TurboVLA: 100) & 220 \\
main Fig.~1, attention rows; \cref{supp:A1n}(b) & OpenVLA-OFT, \piO, \piH & the 5 Task-paired scenes, first frame & 0--9 & 7 & 50 frames per model & -- \\
\cref{supp:Gkv,supp:Gmap} & \piH, \piO & Position; Object tasks 0--9, first frame & 6--15 & -- & 100 frames, 500 name pairs per model & -- \\
main Fig.~3(b, c); \cref{supp:B2,supp:B1} & \piH, \piO & Position, original scenes; tasks 0, 3, 6, 8, 9 & 0--19 & 7, 17 & 200 per cut & 220 \\
\cref{supp:B2}, repeat; \cref{supp:B0chk,supp:B7} & \piH, \piO & Position, original scenes; tasks 0, 3, 6, 8, 9 & 0--49 & 7 & 250 per cut & 280 \\
\cref{supp:G1} & \piH & Position; tasks 0, 9 & 0--49 & 7 & 50 per cell and task & 280 \\
main Fig.~4 & \piH, PSG & Position; Object task 6 (butter) & 13 & 7 & one episode each; 32 samples per query & 280 \\
main Fig.~5(a); \cref{supp:C3} & \piH & Position; 5 Object tasks & 6--15 & 7 & 10 frames per object & -- \\
main Fig.~5(b) & \piH, PSG, each effect alone & Position; Object tasks 0, 3, 6 & 0--49 & 7 & 50 per task and row & 280 \\
\cref{supp:C3}, Reach axis & \piH, PSG & Position; Object tasks 0, 3, 6, 8, 9 & 0--49 & 7 & 50 per task & 280 \\
main Tab.~1; \cref{supp:C5,supp:D1,supp:D1b,supp:D1c} & the methods of \cref{supp:D3} & LIBERO, LIBERO-PRO & 0--49 & 7 & 50 per task & 220--520 \\
main Tab.~1, Layout column & the methods of \cref{supp:D3} & LIBERO-Plus Layout, 1,525 tasks & 0 & 7 & one per task & 220--520 \\
main Tab.~2, Fig.~7; \cref{supp:C2,supp:D1e}; \cref{supp:protocol-text} & the methods of \cref{supp:D3} & LIBERO-Object and LIBERO-Goal, object moved & 6--15 & 7 & 689 (Object), 210 (Goal) per method & 280--300 \\
main Tab.~3; \cref{supp:D1f} & the methods of \cref{supp:D3} & LIBERO-CF & 0--49 & 7 & 50 per task & 220--280 \\
\cref{supp:C4p2,supp:C4p2fig} & \piH, PSG's sampler & Position; Object tasks 0--9 & 0--5,\,16--29 & 7 & 200 per row & 280 \\
\cref{supp:C6} & \piH, \piO, PSG & Position; Object tasks 0--9 & 0--49 & 7, 17 (\piO: 7) & 500 per row & 280 \\
\cref{supp:protocol-text}, selection & \piH, PSG & 11 development tasks & 6--15 & 7, 17 & 110 per condition and seed & -- \\
main Fig.~2; \cref{supp:A1n}(a); \cref{supp:A4,supp:A5} & three stages per lineage & 126 scenes, nine objects & two & -- & one frame per scene & -- \\
main Fig.~6(b) & \piH & ten Object tasks' objects, seven places & 6--15 & two & 1,378 & -- \\
\cref{supp:protocol-text}, first close & the methods of \cref{supp:D3} & every test set of \cref{supp:D2}, pooled & \multicolumn{4}{l}{as in \cref{supp:D2}} \\
\bottomrule
\end{tabular}
