# Supplementary material for: Seeing Is Not Reaching: Instruction Shortcuts Override Visual Grounding in Vision-Language-Action Models
Source: arXiv:2611.32206 source file (2026-11-24)
Supplement: Supplementary file 41 [file float.tex]

\begin{table*}[tp]
\centering
\setlength\heavyrulewidth{0.25ex}
\footnotesize
\setlength{\tabcolsep}{3pt}
\captionsetup{position=top,skip=4pt}
\caption{\textbf{The settings behind each figure and table.}
Per figure or table of the main paper and of this supplement; steps after the ten settling steps; the checkpoints are in \cref{supp:D3}; --: no rollout, or not stated.}
\label{supp:D3runs}\label{supp:D3passes}
\input{sec/suppl/D3runs/D3settings_tabular.tex}
\end{table*}
