# Supplementary material for: Seeing Is Not Reaching: Instruction Shortcuts Override Visual Grounding in Vision-Language-Action Models
Source: arXiv:2611.32206 source file (2026-11-24)
Supplement: Supplementary file 42 [file algorithm.tex]

\makeatletter
\@ifundefined{c@algobox}{%
\newcounter{algobox}%
\renewcommand{\thealgobox}{S\arabic{algobox}}%
\renewcommand{\theHalgobox}{S\arabic{algobox}}%
\def\fps@algobox{tbp}%
\def\ftype@algobox{8}%
\def\ext@algobox{loa}%
\def\fnum@algobox{Algorithm~\thealgobox}%
\def\algoboxname{Algorithm}%
\newenvironment{algobox}{\@float{algobox}}{\end@float}}{}
\makeatother
\par\medskip\noindent\begin{minipage}{\linewidth}\makeatletter\def\@captype{algobox}\makeatother
\centering
\captionsetup{position=top,skip=4pt}
\caption{Pathway-Separated Guidance: sampling one action chunk.}
\label{alg:psg}
\small
\setlength{\tabcolsep}{2pt}
\begin{tabular}{@{}r@{\hspace{6pt}}p{0.86\linewidth}@{}}
\toprule
\multicolumn{2}{@{}p{0.97\linewidth}@{}}{\textbf{Input:} observation $\mathbf{o}_t$ (main- and wrist-camera images, instruction $\ell$); name tokens $N\subset\ell$; weights $a,b$ (PSG: $a,b\ge 0$; \cref{supp:C4p2} also runs the sampler at $a=-1$); number of Euler steps $K$, step size $\delta=1/K$.}\\
\midrule
1: & Encode the prefix with the full attention mask; keep its key--value cache $\mathcal{C}$.\\
2: & Encode the prefix again with $I_m\nrightarrow N$; keep its cache $\mathcal{C}_g$.\\
3: & Sample $\mathbf{A}_t^0\sim\mathcal{N}(\mathbf{0},\mathbf{I})$; set $\tau\leftarrow 0$.\\
4: & \textbf{while} $\tau<1$ \textbf{do}\\
5: & \quad $v\leftarrow v_\theta(\mathbf{A}_t^\tau,\mathbf{o}_t)$, action tokens reading $\mathcal{C}$\\
6: & \quad $v[I_m\nrightarrow N]\leftarrow$ the same, reading $\mathcal{C}_g$\\
7: & \quad $v[A\nrightarrow\ell]\leftarrow$ the same, reading $\mathcal{C}$ without $\ell$\\
8: & \quad $v_g\leftarrow v-v[I_m\nrightarrow N]$,\quad $v_d\leftarrow v-v[A\nrightarrow\ell]$\\
9: & \quad $\tilde v\leftarrow v+a\,v_g-b\,v_d$ on the six motion dimensions\\
10: & \quad $\tilde v\leftarrow v$ on the gripper dimension\\
11: & \quad $\mathbf{A}_t^{\tau+\delta}\leftarrow\mathbf{A}_t^\tau+\delta\,\tilde v$;\quad $\tau\leftarrow\tau+\delta$\\
12: & \textbf{end while}\\
13: & \textbf{return} $\mathbf{A}_t^1$\\
\bottomrule
\end{tabular}
\end{minipage}\par\medskip
