# Supplementary material for: Seeing Is Not Reaching: Instruction Shortcuts Override Visual Grounding in Vision-Language-Action Models
Source: arXiv:2611.32206 source file (2026-11-24)
Supplement: Supplementary file 43 [file D5_tabular.tex]

\footnotesize
\setlength{\tabcolsep}{2.1pt}
\begin{tabular}{lrrrrrrr}
\toprule
 & \multicolumn{1}{c}{Prefix} & \multicolumn{3}{c}{Action expert} & Actions & \multicolumn{2}{c}{Time}\\
\cmidrule(lr){2-2}\cmidrule(lr){3-5}\cmidrule(lr){7-8}
Method & \ml{passes} & \ml{per step} & \ml{steps} & \ml{passes} & \ml{executed} & \ml{s / query} & \ml{h / 500}\\
\midrule
\piH & 1 & 1 & 10 & 10 & 5 & 0.154--0.172 & 1.2--1.3\\
\piH\ + CAG & 2 & 2 & 10 & 20 & 5 & 0.237 & 1.8\\
\rowcolor[HTML]{EDEDED}\piH\ + PSG & 2 & 3 & 10 & 30 & 5 & 0.245--0.257 & 1.9--2.0\\
\bottomrule
\end{tabular}
