# Supplementary material for: Seeing Is Not Reaching: Instruction Shortcuts Override Visual Grounding in Vision-Language-Action Models
Source: arXiv:2611.32206 source file (2026-11-24)
Supplement: Supplementary file 44 [file float.tex]

\begin{table}[tbp]
\centering
\setlength\heavyrulewidth{0.25ex}
\captionsetup{position=top,skip=4pt}
\caption{\textbf{Cost per action chunk.} Backbone passes over the images and the instruction (prefix) and action-expert passes, for the released policy, with CAG and with PSG. Seconds per query measured in short trials on one 24\,GB card; the hours per 500 LIBERO-PRO Position Object episodes follow from it with every episode run to the step limit, an upper bound.}
\label{supp:D5}
\input{sec/suppl/D5/D5_tabular.tex}
\end{table}
