# Supplementary material for: Seeing Is Not Reaching: Instruction Shortcuts Override Visual Grounding in Vision-Language-Action Models
Source: arXiv:2611.32206 source file (2026-11-24)
Supplement: Supplementary file 45 [file D6_tabular.tex]

\begin{tabular}{lllllll}
\toprule
\parbox[t]{1.9cm}{\raggedright\strut Figure or table\strut} & \parbox[t]{2.15cm}{\raggedright\strut Tokens $\to$ camera\strut} & \parbox[t]{2.2cm}{\raggedright\strut Averaged over\strut} & \parbox[t]{2.15cm}{\raggedright\strut When\strut} & \parbox[t]{2.0cm}{\raggedright\strut Patches\strut} & \parbox[t]{2.6cm}{\raggedright\strut Statistic\strut} & \parbox[t]{3.2cm}{\raggedright\strut Scenes and N\strut} \\
\midrule
\parbox[t]{1.9cm}{\raggedright\strut Main Fig.~2(b); \cref{supp:A1n}(a); \cref{supp:A5}\strut} & \parbox[t]{2.15cm}{\raggedright\strut name $\to$ main camera\strut} & \parbox[t]{2.2cm}{\raggedright\strut all layers and heads (\piH: 18 $\times$ 8)\strut} & \parbox[t]{2.15cm}{\raggedright\strut one pass on the start frame; wrist image blank\strut} & \parbox[t]{2.0cm}{\raggedright\strut every patch the object touches, equal weight\strut} & \parbox[t]{2.6cm}{\raggedright\strut $\div$ image average; per object the median over its scenes; geometric mean over 9 objects\strut} & \parbox[t]{3.2cm}{\raggedright\strut 9 objects at 6 new places, 2 start states: 108 moved scenes, 18 at the training place\strut} \\ \addlinespace[4pt]
\parbox[t]{1.9cm}{\raggedright\strut Main Fig.~2(a); \cref{supp:A4}\strut} & \parbox[t]{2.15cm}{\raggedright\strut name $\to$ main camera\strut} & \parbox[t]{2.2cm}{\raggedright\strut as above\strut} & \parbox[t]{2.15cm}{\raggedright\strut as above\strut} & \parbox[t]{2.0cm}{\raggedright\strut as above\strut} & \parbox[t]{2.6cm}{\raggedright\strut share of the name's attention on a set of patches (\%); medians over the 12 moved scenes\strut} & \parbox[t]{3.2cm}{\raggedright\strut as above\strut} \\ \addlinespace[4pt]
\parbox[t]{1.9cm}{\raggedright\strut \cref{supp:A1n}(b); main Fig.~1, name row\strut} & \parbox[t]{2.15cm}{\raggedright\strut name $\to$ main camera\strut} & \parbox[t]{2.2cm}{\raggedright\strut 18 $\times$ 8 (OpenVLA-OFT: 32 $\times$ 32)\strut} & \parbox[t]{2.15cm}{\raggedright\strut first policy frame; real wrist image\strut} & \parbox[t]{2.0cm}{\raggedright\strut weighted by the object's pixels\strut} & \parbox[t]{2.6cm}{\raggedright\strut $\div$ image average; median over frames\strut} & \parbox[t]{3.2cm}{\raggedright\strut the 5 Task-paired pairs, start states 0--9, noise seed 7: 50 frames\strut} \\ \addlinespace[4pt]
\parbox[t]{1.9cm}{\raggedright\strut Main Fig.~1, action row\strut} & \parbox[t]{2.15cm}{\raggedright\strut action $\to$ main camera (OpenVLA-OFT: its 56 action positions)\strut} & \parbox[t]{2.2cm}{\raggedright\strut $\pi$ models: Euler steps, layers, heads, action tokens; OpenVLA-OFT: 32 $\times$ 32 layers and heads\strut} & \parbox[t]{2.15cm}{\raggedright\strut first policy frame; real wrist image\strut} & \parbox[t]{2.0cm}{\raggedright\strut weighted by the object's pixels\strut} & \parbox[t]{2.6cm}{\raggedright\strut $\div$ image average; median over frames\strut} & \parbox[t]{3.2cm}{\raggedright\strut the same 50 frames; \piH, \piO\ and OpenVLA-OFT\strut} \\ \addlinespace[4pt]
\parbox[t]{1.9cm}{\raggedright\strut Main Fig.~3(c); \cref{supp:B6}\strut} & \parbox[t]{2.15cm}{\raggedright\strut action $\to$ main camera\strut} & \parbox[t]{2.2cm}{\raggedright\strut 8 heads, the action tokens (10 in \piH, 50 in \piO), 18 layers, 10 Euler steps\strut} & \parbox[t]{2.15cm}{\raggedright\strut first query\strut} & \parbox[t]{2.0cm}{\raggedright\strut every patch the object touches, equal weight\strut} & \parbox[t]{2.6cm}{\raggedright\strut $\div$ image average; median and quartiles over episodes\strut} & \parbox[t]{3.2cm}{\raggedright\strut LIBERO-PRO Position, 5 tasks, start states 0--19, noise seeds 7 and 17: 200 episodes per cut\strut} \\ \addlinespace[4pt]
\parbox[t]{1.9cm}{\raggedright\strut Main Fig.~5(a); \cref{supp:C3}\strut} & \parbox[t]{2.15cm}{\raggedright\strut name $\to$ main camera\strut} & \parbox[t]{2.2cm}{\raggedright\strut the name's tokens, 18 $\times$ 8\strut} & \parbox[t]{2.15cm}{\raggedright\strut first query; both cameras' images\strut} & \parbox[t]{2.0cm}{\raggedright\strut weighted by the object's pixels\strut} & \parbox[t]{2.6cm}{\raggedright\strut per frame: own name $\div$ highest of the other names; median over frames\strut} & \parbox[t]{3.2cm}{\raggedright\strut LIBERO-PRO Position, 5 tasks, start states 6--15, noise seed 7: 10 frames per object\strut} \\ \addlinespace[4pt]
\parbox[t]{1.9cm}{\raggedright\strut Main Fig.~6(b)\strut} & \parbox[t]{2.15cm}{\raggedright\strut name and action $\to$ main and wrist camera\strut} & \parbox[t]{2.2cm}{\raggedright\strut 18 $\times$ 8\strut} & \parbox[t]{2.15cm}{\raggedright\strut six commands of each episode (0, 5, 10, 15, 20, 30)\strut} & \parbox[t]{2.0cm}{\raggedright\strut the object's patches in that camera\strut} & \parbox[t]{2.6cm}{\raggedright\strut $\div$ that camera's average; median per distance bin, ten objects and all places pooled\strut} & \parbox[t]{3.2cm}{\raggedright\strut the LIBERO-Object objects at their training place and six new places, start states 6--15, noise seeds 7 and 17: 1,378 episodes of the released \piH, 8,268 observations, 8,132 of them in the main camera's bins\strut} \\
\bottomrule
\end{tabular}
