# Supplementary material for: Seeing Is Not Reaching: Instruction Shortcuts Override Visual Grounding in Vision-Language-Action Models
Source: arXiv:2611.32206 source file (2026-11-24)
Supplement: Supplementary file 46 [file float.tex]

\begin{table*}[tp]
\centering
\footnotesize
\setlength\heavyrulewidth{0.25ex}
\setlength{\tabcolsep}{2.5pt}
\captionsetup{position=top,skip=4pt}
\caption{\textbf{How every attention number of the main paper and the supplementary is computed.}
One line per figure or table: whose attention is read, what it is averaged over, when, on which patches, and the statistic, which gives the line's normalisation. A camera has 256 patches (SmolVLA: 64).}
\label{supp:D6}
\input{sec/suppl/D6/D6_tabular.tex}
\end{table*}
