# Supplementary material for: Seeing Is Not Reaching: Instruction Shortcuts Override Visual Grounding in Vision-Language-Action Models
Source: arXiv:2611.32206 source file (2026-11-24)
Supplement: Supplementary file 47 [file G1_caption.tex]

\caption{\textbf{\boldmath Read through \piH's direct pathway, an instruction draws first closes to its own training place: the scene's on the alphabet soup, a second object's on the orange juice.} Rows: what the image tokens read, the scene's instruction or nothing (the grounding cut); columns: what the action tokens read, the scene's instruction, a second object's instruction or nothing (the direct cut); 50 episodes per cell under LIBERO-PRO Position. Each bar: the episodes by the object the first close lands on, named by where it stood; hatched: the object at the slot beside a training place.}
