# Supplementary material for: Seeing Is Not Reaching: Instruction Shortcuts Override Visual Grounding in Vision-Language-Action Models
Source: arXiv:2611.32206 source file (2026-11-24)
Supplement: Supplementary file 48 [file G1len_tabular.tex]

\begin{tabular}[t]{lrrr}
\toprule
Instruction length, task 9 & \ml{median} & \ml{largest} & \ml{$>$10\%} \\
\midrule
motion dimensions & 0.00684 & 0.0191 & 0 of 50 \\
gripper dimensions & 0.00195 & 0.00293 & 0 of 50 \\
\bottomrule
\end{tabular}
