# Supplementary material for: Seeing Is Not Reaching: Instruction Shortcuts Override Visual Grounding in Vision-Language-Action Models
Source: arXiv:2611.32206 source file (2026-11-24)
Supplement: Supplementary file 49 [file float.tex]

\begin{figure*}[tp]
\centering
\includegraphics[width=\linewidth]{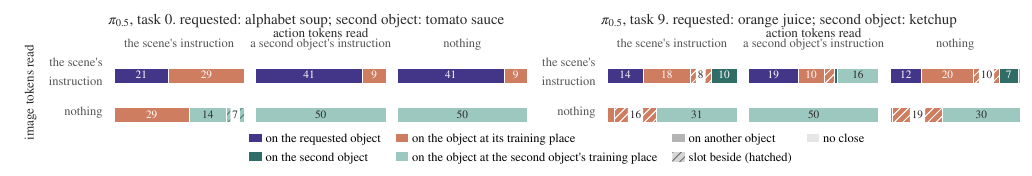}
\input{sec/suppl/G1/G1_caption.tex}
\label{supp:G1}
\end{figure*}
