# Supplementary material for: Seeing Is Not Reaching: Instruction Shortcuts Override Visual Grounding in Vision-Language-Action Models
Source: arXiv:2611.32206 source file (2026-11-24)
Supplement: Supplementary file 50 [file Gkv_caption.tex]

\caption{\textbf{\boldmath In \piH, the named objects' image tokens change more than the rest of the image when the name changes; in \piO, less.}
Mean change per patch of the main-camera image tokens' keys or values on the object's patches when only the requested object's name is replaced, over the mean on the patches that hold neither object; median over the ten tasks with [min--max] (protocol in \cref{supp:protocol-text}).}
