# Supplementary material for: Seeing Is Not Reaching: Instruction Shortcuts Override Visual Grounding in Vision-Language-Action Models
Source: arXiv:2611.32206 source file (2026-11-24)
Supplement: Supplementary file 51 [file Gkv_tabular.tex]

\begin{tabular}{@{}ll cc cc@{}}
\toprule
 & & \multicolumn{2}{c}{keys} & \multicolumn{2}{c}{values} \\
\cmidrule(lr){3-4}\cmidrule(l){5-6}
 & \mlh{layers} & \mlh{requested\\object / rest} & \mlh{substitute\\/ rest} & \mlh{requested\\object / rest} & \mlh{substitute\\/ rest} \\
\midrule
\piH & 1--5 & 1.88 & 1.94 & 1.89 & 1.99 \\
 & & {\scriptsize\color{gray}[1.67--2.65]} & {\scriptsize\color{gray}[1.65--2.18]} & {\scriptsize\color{gray}[1.72--2.84]} & {\scriptsize\color{gray}[1.70--2.26]} \\
\addlinespace[1.5pt]
 & 6--11 & 1.65 & 1.94 & 1.66 & 1.78 \\
 & & {\scriptsize\color{gray}[1.28--3.08]} & {\scriptsize\color{gray}[1.51--2.26]} & {\scriptsize\color{gray}[1.28--2.48]} & {\scriptsize\color{gray}[1.49--1.99]} \\
\addlinespace[1.5pt]
 & 12--17 & 1.62 & 1.84 & 1.71 & 1.73 \\
 & & {\scriptsize\color{gray}[1.17--2.89]} & {\scriptsize\color{gray}[1.52--2.14]} & {\scriptsize\color{gray}[1.27--2.30]} & {\scriptsize\color{gray}[1.59--2.18]} \\
\midrule
\piO & 1--5 & 0.47 & 0.53 & 0.43 & 0.49 \\
 & & {\scriptsize\color{gray}[0.36--0.89]} & {\scriptsize\color{gray}[0.41--0.63]} & {\scriptsize\color{gray}[0.32--0.87]} & {\scriptsize\color{gray}[0.38--0.59]} \\
\addlinespace[1.5pt]
 & 6--11 & 0.46 & 0.52 & 0.42 & 0.48 \\
 & & {\scriptsize\color{gray}[0.39--0.82]} & {\scriptsize\color{gray}[0.41--0.55]} & {\scriptsize\color{gray}[0.34--0.86]} & {\scriptsize\color{gray}[0.37--0.54]} \\
\addlinespace[1.5pt]
 & 12--17 & 0.43 & 0.48 & 0.39 & 0.44 \\
 & & {\scriptsize\color{gray}[0.31--0.65]} & {\scriptsize\color{gray}[0.43--0.53]} & {\scriptsize\color{gray}[0.28--0.60]} & {\scriptsize\color{gray}[0.40--0.49]} \\
\bottomrule
\end{tabular}
