# Supplementary material for: Seeing Is Not Reaching: Instruction Shortcuts Override Visual Grounding in Vision-Language-Action Models
Source: arXiv:2611.32206 source file (2026-11-24)
Supplement: Supplementary file 53 [file Gmap_caption.tex]

\caption{\textbf{\boldmath In \piH, the change of the name lands on the named objects' image tokens; in \piO, it lands elsewhere in the image.}
Left: the main-camera frame of the alphabet soup task under Position, start state 6. Middle and right: the change of each main-camera image token's keys when the requested object's name is replaced by another object's, averaged over the five substitutes and over layers 1--17, relative to its mean over the image; one colour scale, clipped at both ends. Solid outline: the requested object's patches; dashed: the substitutes' patches.}
